# Supplementary material for: Value Function Approximations via Kernel Embeddings for No-Regret Reinforcement Learning
Source: arXiv:2011.07881 source file (2022-06-28)
Supplement: Supplementary file 1 [file Appendix_C.tex]

\section{Extra}

\paragraph{covariance operator}
Further, for any $f,g \in \cH_\psi$, the
mapping $(f,g) \mapsto \C_{X \sim P(\cdot|s,a)}[f(X),g(X)]$ has a bounded bilinear
form. Hence, there exists a unique operator $\Sigma_P^{(s,a)} \in \cL(\cH_\psi,\cH_\psi)$, for each state-action pair $(s,a)$, such
that
\beqn
\forall f,g \in \cH_\psi,\quad \C_{X \sim P(\cdot|s,a)}[f(X),g(X)] = \inner{f}{\Sigma_P^{(s,a)}g}_{k_\psi}~.
\eeqn
We call $\Sigma_P^{(s,a)}$ the kernel covariance operator of the conditional distribution $P(\cdot|s,a)$ and it can be explicitly expressed as\footnote{$f \otimes g$ denotes the tensor product between $f \in \cH_\psi$ and $g \in \cH_\phi$, and for any $h \in \cH_\psi$ satisfies $(f\otimes g)h=\inner{g}{h}_{k_\psi} f$. An analogous result applies for $f,g,h \in \cH_\psi$.
}
\beqn
\Sigma_P^{(s,a)} = \C_{X \sim P(\cdot|s,a)}[\psi(X),\psi(X)]= \esp\left[\psi(X)\otimes \psi(X)\right]-\esp\left[\psi(X)\right]\otimes \esp\left[\psi(X)\right]~.
\eeqn
We will assume that the covariance operators $\Sigma_{P}^{(s,a)}$ are known and only the mean embeddings $\cme_P^{(s,a)}$ need to be estimated from data. Furthermore, boundedness of $k_\psi$ implies that $\Sigma_P^{(s,a)} \preceq B_\psi^2 \eye$, since
\beqn
\norm{\Sigma_P^{(s,a)}} \leq \tr\left[\Sigma_P^{(s,a)}\right] = \esp\left[\norm{\psi(X)}_{k_\psi}^2\right] - \norm{\esp[\psi(X)]}_{k_\psi}^2 \leq B_\psi^2~.
\eeqn

\paragraph{assumptions}

For any two distributions $P,Q:\cS \times \cA \to \Delta(\cS)$ and a function class $\cF : \cS \to \Real$, the \emph{integral probability metrics} ($\IPM$) for each state-action pair $(s,a)$ is defined as
\beqn
\IPM^{(s,a)}_{P,Q}(\cF) := \sup_{f \in \cF}\abs{\Esp_{X \sim P(\cdot | s,a)}[f(X)]-\Esp_{X \sim Q(\cdot | s,a)}[f(X)]}~.
\eeqn
When $\cF = \lbrace f \in \cH_\psi : \norm{f}_{k_\psi} \leq 1 \rbrace$, the $\IPM$ is equal to the \emph{maximum mean discrepancy} ($\MMD$) defined as
\beqn
\MMD^{(s,a)}_{P,Q} := \norm{\cme_P^{(s,a)}-\cme_Q^{(s,a)}}_{k_\psi}~.
\eeqn

\begin{myassumption}[Smooth transition structure]
For the function class $\cF = \lbrace f: \norm{f}_{\infty} \leq 1 \rbrace$, it holds
for all $(s,a) \in \cS \times \cA$ that $\IPM^{(s,a)}_{P,Q}(\cF) \leq c \cdot \MMD^{(s,a)}_{P,Q}$
for some problem dependent constant $c > 0$ .
\label{ass:IPM-MMD-equivalence}
\end{myassumption}
 
\begin{mycorollary}[Regret bound under Assumption \ref{ass:IPM-MMD-equivalence}] For any $\delta \in (0,1]$, the following holds with probability at least $1-\delta :$
\beqn
\cR(N) = \Otilde{c\cdot\gamma_{\phi,T}^{\lambda}\sqrt{H^3N\log(1/\delta)}}~.
\eeqn

% \beqn
% \cR(N) \leq  2cH\beta_T \sqrt{2(1+\lambda^{-1}B_\phi^2 H)N\gamma_{\phi,T}^{\lambda}}  + 2H\sqrt{2N\log(2/\delta)}~,
% \eeqn
% where $\beta_T=\sqrt{\lambda}B+2B_\psi\sqrt{2\left(\log(2/\delta)+\gamma_{\phi,T-1}^{\lambda}\right)}$.
\label{cor:regret-IPM-MMD-equivalence}
\end{mycorollary}

\begin{myexample}[Non-linear dynamics with Gaussian noise] Suppose the transition model follows the non-linear dynamical system \citep{kakade2020information} evolution given by $s' =  W \phi(s,a) + \zeta$, 	
where $W : \cH_{\phi} \to \cS \subset \Real^m$ is a unknown linear mapping and $\zeta \!\sim\! \mathcal{N}(0,\sigma^2 \eye)$ is i.i.d. noise.\footnote{This model admits the linear dynamics (Example \ref{ex:LDS}) as a special case.} In this case, by an application of Pinsker's inequality, Assumption \ref{ass:IPM-MMD-equivalence} holds with $c=1/2\sigma$. 
\label{ex:NLDS}
\end{myexample}

\begin{myremark}
For the model in Example \ref{ex:NLDS}, our regret bound matches the bound given in \citet{kakade2020information} in terms of scaling with $\gamma_{\phi,T}^{\lambda}$, $H$ and $N$. Moreover, our bound is independent of the dimension $m$ of the state space, whereas their bound scales as 
$O(\sqrt{m})$. This improvement is a consequence of our novel concentration inequality for the mean embeddings (Lemma \ref{lem:concentration}).
Further, their bound has improved dependencies on problem dependent parameters $B$, $B_\phi$ and $\sigma$. However, we believe that it is a consequence of their tailor made analysis for Gaussian densities whereas our analysis works for any distribution satisfying Assumption \ref{ass:IPM-MMD-equivalence}, Gaussian being an example.
\end{myremark}

\begin{myremark}
Assumption \ref{ass:IPM-MMD-equivalence} implies that if the mean embeddings of two distributions are close in the RKHS distance, then their total variation distance is small. A conceptually similar assumption involving the centered transition distributions in the place of mean embeddings have been considered in prior works \citep{osband2014model,chowdhury2019online}; however the results are not directly comparable.
\end{myremark}

\begin{myassumption}
For any $f: \cS \to \Real$, there exists a $w_f \in \cH_{\psi}$ with $\norm{w_f}_{k_\psi} \leq c_\psi$ such that
$\Esp_{X \sim P(\cdot | s,a)}[f(X)] = \inner{w_f}{ \cme_P^{(s,a)}}_{k_\psi}~$.
\label{ass:almost-opt-closure}
\end{myassumption}
This assumption effectively implies that the transition distribution appears to be linear in the space of mean embeddings when applied to the value functions obtained using optimistic Bellman updates (\autoref{eq:optimistic-values}).

\begin{myremark}
For the function class in Assumption \ref{ass:almost-opt-closure}, Assumption \ref{ass:IPM-MMD-equivalence} holds with $c=c_\psi$ and hence, the bound given in Corollary \ref{cor:regret-IPM-MMD-equivalence} also holds in this case. However, the converse is not always true. For example, Assumption \ref{ass:almost-opt-closure} doesn't necessarily hold for the non-linear dynamics in Example \ref{ex:NLDS}.
\end{myremark}

% \begin{mycorollary}[Regret bound under Assumption \ref{ass:almost-opt-closure}]
% For any $\delta \in (0,1]$, the following holds with probability at least $1-\delta :$
% \beqn
% \cR(N) \leq  2c_{\psi}H\beta_T \sqrt{2(1+\lambda^{-1}B_\phi^2 H)N\gamma_{\phi,T}^{\lambda}}  + 2H\sqrt{2N\log(2/\delta)}~,
% \eeqn
% where $\beta_T=\sqrt{\lambda}B+2B_{\psi}\sqrt{2\left(\log(2/\delta)+\gamma_{\phi,T-1}^{\lambda}\right)}$.
% \label{cor:regret-almost-opt-closure}
% \end{mycorollary}

\begin{myexample}[Bilinear transitions]
Suppose the transition probabilities are given by the bilinear form $P(s'|s,a) = \psi(s')^\top \Theta_P\phi(s,a)$, where $\psi:\cS\to\Real^p$ and $\phi:\cS\times\cA \to \Real^q$ are known feature functions, and $\Theta_P$ is a $p\times q$ matrix of unknown parameters \citep{yang2019reinforcement}. In this case, Assumption \ref{ass:almost-opt-closure} holds with $\cH_\psi=\Real^p$, $\cH_\phi=\Real^q$ and $w_f=\int_{\cS}f(s')\psi(s')\diff s' \in \Real^p$, where the integral is taken component-wise.
\label{ex:bilinear-transition}
\end{myexample}

\begin{myremark}
For the model in Example \ref{ex:bilinear-transition}, the information gain $\gamma_{\phi,T}^{\lambda}$ scales as $O(q \log N)$. In this case, we obtain a regret bound of $\tilde{O}(q\sqrt{H^3N})$ that is $O(\sqrt{H})$ factor better than \citet[Theorem 2]{yang2019reinforcement} and is a consequence of a tighter bound on sum of predictive variances (Lemma \ref{lem:sum-of-predictive-variances}) compared to \citet{yang2019reinforcement}. Furthermore, they need $\Theta_P$ to be Hilbert-Schmidt, whereas we only need a weaker boundedness assumption. This is achieved through a tighter concentration result ($O(\log N)$ improvement over \citet{yang2019reinforcement}) of the mean embedding operator (Lemma \ref{lem:concentration}).
\end{myremark}

\begin{myremark}
For the model in Example \ref{ex:bilinear-transition}, the $Q$ updates given by \autoref{eq:optimistic-planning} can be replaced by the following closed form expression keeping the regret guarantees intact:
\beqn
Q_h^t(s,a) = R(s,a) + \left(\vec k_{\phi,t}^{(s,a)}\right)^\top (\mat K_{\phi,t}+\lambda \eye)^{-1}\vec w^t_{h+1} + c_\psi\beta_t\lambda^{-1/2} \sigma_{\phi,t}(s,a)~,
\eeqn
where the $(\tau',h')$-th element ($\tau' < t$, $h' \leq H$) of the vector $\vec w^t_{h+1} \in \Real^n$ is given by $\sum_{s \in \cS}V_{h+1}^{t}(s)k_{\psi}(s_{h'+1}^{\tau'},s)$ and the constant $c_\psi$ is a uniform upper bound over $\norm{\sum_{s \in \cS}V_{h+1}^{t}(s)\psi(s')}_{k_\psi}$ for all $t$ and $h$. Note that our $Q$ updates in this case are different than that of \citet{yang2019reinforcement}, but much like them, we also need access to an efficient sampler in the state space.
\end{myremark}

\begin{myremark}
For the class of value functions in Assumption \ref{ass:opt-closure}, both Assumptions \ref{ass:almost-opt-closure} and \ref{ass:IPM-MMD-equivalence} hold and hence, the bound given in Corollary \ref{cor:regret-IPM-MMD-equivalence} also holds with $c=v_\psi$ .
\end{myremark}

\begin{myremark}
% Since the value estimates lies in $\cH_\psi$, we can write
% \beqan
% \esp_{X \sim P'(\cdot | s,a)}\left[V_{h+1}^{t}(X)\right] &=& \inner{V_{h+1}^t}{\hat\cme_t^{(s,a)}}_{k_\psi}+ \inner{V_{h+1}^t}{\cme_{P'}^{(s,a)}-\hat\cme_t^{(s,a)}}_{k_\psi}\\
% & \leq & \inner{V_{h+1}^t}{\hat\cme_t^{(s,a)}}_{k_\psi} + \norm{V_{h+1}^t}_{k_\psi}\beta_t\lambda^{-1/2} \sigma_{\phi,t}(s,a)~.
% \eeqan

\end{myremark}
